# Supplementary material for: Maximally-localized Wannier orbitals and the extended Hubbard model for the twisted bilayer graphene
Source: arXiv:1805.06819 ancillary file (2018-08-06)
Supplement: Supplementary file 1 [file SupplMaterial.pdf]

# Supplementary Material for "Maximally-localized Wannier orbitals and the extended Hubbard model for the twisted bilayer graphene": Wannier orbitals in twisted bilayer graphene with different point groups

Mikito Koshino,[1] Noah F. Q. Yuan,[2] Takashi Koretsune,[3] Masayuki Ochi,[1] Kazuhiko Kuroki,[1] and Liang Fu[2]

[1]*Department of Physics, Osaka University, Toyonaka 560-0043, Japan*
[2]*Department of Physics, Massachusetts Institute of Technology, Cambridge, Massachusetts 02139, USA*
[3]*Department of Physics, Tohoku University, Sendai 980-8578, Japan*

In this part of Supplementary Material we consider symmetries and centers of Wannier orbitals in different superlattice structures of twisted bilayer graphene (TBG). For monolayer graphene we find three types of high-symmetry points: carbon atoms, carbon-bond midpoints and hexagon centers. We start from AA stacking where all three types of high-symmetry points in two layers are registered.

| | $\bar{\Gamma}$ | $\bar{K}$ | $\bar{M}$ | Orbitals | Lattice |
|---|---|---|---|---|---|
| Group | $C_2$ | $C_2$ | $C_2$ | $C_2$ | Triangular |
| Reps | $\{A, B; A, B\}$ | $\{A, B; A, B\}$ | $\{A, B; A, B\}$ | $\{s, p; s, p\}$ | |
| Group | $D_2$ | $C_2$ | $D_2$ | $D_2$ | Triangular |
| Reps | $\{A, B_1; B_2, B_3\}$ | $\{A, B; A, B\}$ | $\{A, B_1; B_2, B_3\}$ | $\{s, p_x; p_y, p_z\}$ | |
| Group | $D_3$ | $D_3$ | $C_2$ | $C_3$ | Honeycomb |
| Reps | $\{E; E\}$ | $\{A_1, A_2, E\}$ | $\{A, B; A, B\}$ | $(p_x, p_y)$ | |
| Group | $D_6$ | $D_3$ | $D_2$ | $D_3$ | Honeycomb |
| Reps | $\{A_1, B_1; A_2, B_2\}$ | $\{E; E\}$ | $\{A, B_1; B_2, B_3\}$ | $\{s, p_z\}$ | |

TABLE I: Symmetries and band orderings of lowest four eigenstates at $\bar{\Gamma}, \bar{K}, \bar{M}$ points for different superlattice structures of TBG. Wannier orbitals (Orbitals) and lattices (Lattice) in effective tight-binding models are also shown. At each high symmetry point, the little group (Group) and irreducible representations (Reps) of the lowest four bands are listed. The semicolons are used to indicate the band gap which separates eigenstates. In $D_3$ structure the band structure at $\bar{K}$ point can be gapped or gapless, hence semicolon is not there. For Wannier orbitals, Group is the point group with respect to their centers (AA spots for traingular lattice and AB or BA spots for honeycomb lattice), Reps are real representations furnished by Wannier orbitals. Here $p$ orbital in $C_2$ structure can be $p_x$ or $p_z$, which is odd under $C_{2y}$.

While in the maintext we studied $D_3$ structure, we now develop a comprehensive symmetry analysis for other superlattice structures including $D_6$ structure (Fig. 1) by properly incorporating the underlying lattice within the continuum model approximation.

As pointed out in the maintext, if the hexagon centers of two graphene layers are registered as the origin, then the TBG has two types of registered high-symmetry points: Hexagon center registration (AA spots) and sublattice registration (AB and BA spots) as shown in Fig. 1. With respect to AA spots the point group is $D_6$ with an extra generator of two-fold rotation $C_{2x}$ along $x$-axis. With respect to AB or BA spots, the point group is $D_3$ generated by $C'_{3z}$ and $C_{2x}$. Besides high-symmetry $D_3$ and $D_6$ structures, TBG can also have low-symmetry superlattice structures. When neither carbon atoms nor hexagon centers are registered, with respect to the rotation center of twist (AA spots), the point group can be $D_2$ generated by $C_{2y}$ and $C_{2x}$ if carbon bond midpoints of two layers are registered as the origin, or the point group is $C_2$ generated by $C_{2y}$ if even carbon-bond midpoints are not registered.

The symmetries and band orderings of lowest four eigenstates at $\overline{\Gamma}, \overline{K}, \overline{M}$ points, and Wannier orbitals for $C_2, D_2, D_3$ and $D_6$ structures are summarized in Table. I. Notice that the band orderings are indicated by semicolons.

## I. $D_6$ STRUCTURE

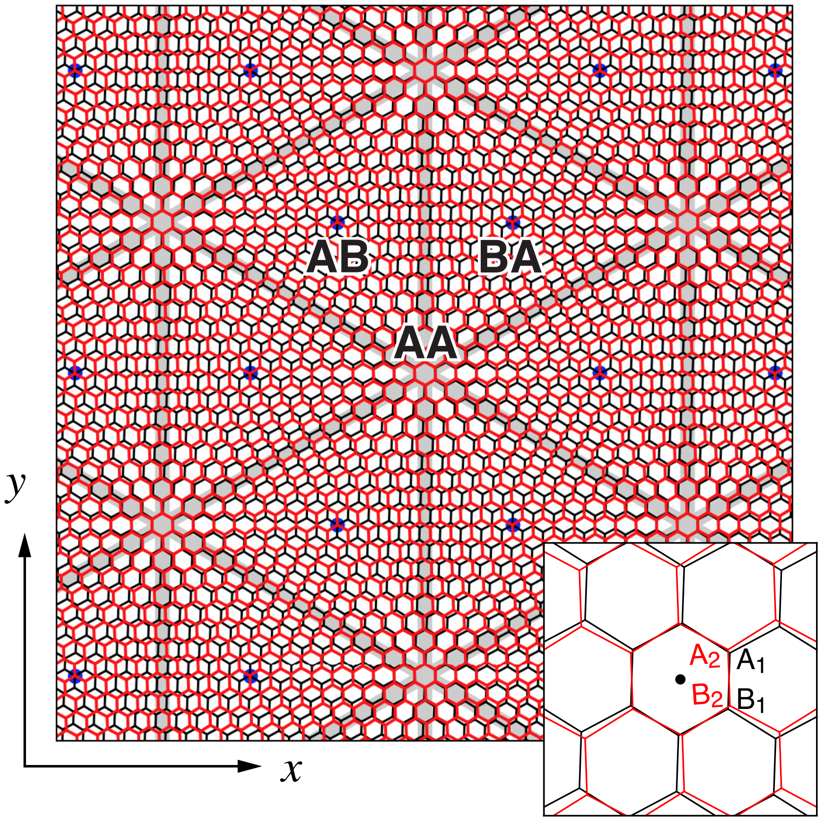


FIG. 1: Atomic structure of TBG with $\theta = 3.89^\circ$ with $D_6$ symmetry.

When the rotation center of TBG is the registered hexagon centers of two layers, the TBG has point group $D_6$ with respect to the rotation center. In this case threefold rotation is preserved, hence the triangular lattice formed by AA spots and the honeycomb lattice formed by AB and BA spots are both candidates for effective tight-binding model. Similar to above structures, in Table. II we list band symmetries in triangular lattice model with different Wannier orbital symmetries, and in Table. III find out the correct effective-tight binding model to reproduce the realistic band symmetries.

| Lattice | Orbitals | $\bar{\Gamma}(D_6)$ | $\bar{K}(D_3)$ | $\bar{M}(D_2)$ | On-site | Orbital U(1) |
|---|---|---|---|---|---|---|
| Honeycomb | $s, f_{x(x^2-3y^2)}$ | $\{A_1; B_1\}$ | $E$ | $\{A; B_1\}$ | $A_1$ | $s \pm i f_{x(x^2-3y^2)}$ |
| $D_3$ | $p_z, f_{y(3x^2-y^2)}$ | $\{A_2; B_2\}$ | $E$ | $\{B_2; B_3\}$ | $A_2$ | $p_z \pm i f_y$ |
| | $(p_x, p_y)$ | $\{E_1; E_2\}$ | $\{A_1, A_2, E\}$ | $\{A, B_1; B_2, B_3\}$ | $E$ | $p_x \pm i p_y$ |
| Triangular | $s$ | $A_1$ | $A_1$ | $A$ | $A_1$ | $s \pm i f_{x(x^2-3y^2)}$ |
| | $f_{x(x^2-3y^2)}$ | $B_1$ | $A_2$ | $B_1$ | $B_1$ | |
| $D_6$ | $p_z$ | $A_2$ | $A_2$ | $B_3$ | $A_2$ | $p_z \pm i f_{y(3x^2-y^2)}$ |
| | $f_{y(3x^2-y^2)}$ | $B_2$ | $A_1$ | $B_2$ | $B_2$ | |
| | $(p_x, p_y)$ | $E_1$ | $E$ | $\{B_1; B_2\}$ | $E_1$ | $p_x \pm i p_y$ |
| | $(d_{x^2-y^2}, d_{xy})$ | $E_2$ | $E$ | $\{A; B_3\}$ | $E_2$ | $d_{x^2-y^2} \pm i d_{xy}$ |

TABLE II: Symmetries of eigenstates at $\bar{\Gamma}$, $\bar{K}$, $\bar{M}$ points for different Wannier orbitals (Orbitals) on different lattices (Honeycomb and Triangular). For honeycomb (triangular) lattice, the on-site symmetry group of Wannier orbitals is $D_3$ ($D_6$), and Wannier orbitals form representations of such on-site symmetry group, which are listed in the column On-site.

From continuum model we know $C_{2y}$ should flip the valley index, and hence the basis constructed for orbital U(1)

| | $\bar{\Gamma}$ | $\bar{K}$ | $\bar{M}$ | Orbitals | Lattice and U(1) |
|---|---|---|---|---|---|
| Group | $D_6$ | $D_3$ | $D_2$ | $D_3$ | Honeycomb |
| Reps | $\{A_1, B_1; A_2, B_2\}$ | $\{E; E\}$ | $\{A, B_1; B_2, B_3\}$ | $\{s, p_z\}$ | NA |

TABLE III: Symmetries and band orderings of lowest four eigenstates at $\bar{\Gamma}, \bar{K}, \bar{M}$ points for $D_6$ structure of TBG. In this case Wannier orbitals cannot implement U(1) symmetry.

symmetry should become complex conjugate under $C_{2y}$. Moreover, from continuum model we know $C_{2x}$ should not flip the valley index, and hence the basis constructed for orbital U(1) symmetry should be eigenstates of $C_{2x}$.

Under conditions from both $C_{2x}, C_{2y}$, the constructed U(1)-symmetric Wannier orbitals in Table. II cannot reproduce realistic band symmetries and band orderings in Table. III, either on a honeycomb or a triangular lattice. And to correctly reproduce band symmetries in Table. III, Wannier orbitals should be singlets with opposite eigenvalues of $C_{2x}$, thus breaking the compatibility between $C_{2x}$ and orbital U(1) symmetry. Furthermore, to reproduce the band ordering in Table. III, the hopping parameters in effective tight-binding model show weird dependence on the distance.

In $D_6$ structure, the effective continuum model has symmetry group $D_6\times$U(1)$\times$SU(2)$\times T$, and the Dirac nodes at $\bar{K}$ and $\bar{K}'$ are protected by this group. In the Hamiltonian of continuum model, $T$ and $C_{2z} \in D_6$ operate on the wave function as

$$T\psi^{X_l}(\mathbf{r}) = \psi^{X_l}(\mathbf{r})^*, \quad C_{2z}\psi^{X_l}(\mathbf{r}) = \psi^{\bar{X}_l}(-\mathbf{r}), \tag{1}$$

where $\bar{X} = B, A$ for $X = A, B$ respectively. $TC_{2z}$ symmetry of continuum model guarantees the band degeneracy at $\bar{K}$ and $\bar{K}'$ in effective continuum model. When including the atomic lattice structure, one can see that $C_{2z}$ exists in the $D_6$ structure (Fig. 1) while not in other structures due to the lack of $C_{6z}$. In other words, the Dirac nodes are symmetry-protected *only* in $D_6$ structure.

To see the microscopic composition of eigenstates at high symmetry points in $D_6$ structure, we study the lowest minibands of TBG at $\bar{\Gamma}, \bar{M}, \bar{K}$ points of the MBZ. In the following we consider leading order contributions from states located closest to the original Dirac points $\pm\boldsymbol{K}_{1,2}$ of individual graphene layers. Compare with the maintext, $\boldsymbol{K}_\xi^{(l)} = -\xi\boldsymbol{K}_l$ for $\xi = \pm$ and $l = 1, 2$.

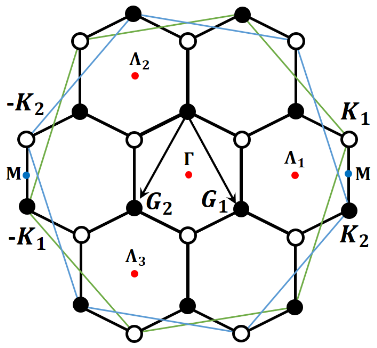


FIG. 2: Mini Brillouin zone (MBZ) of twisted bilayer graphene with rotation angle $\theta = 21.8°$. Blue and green large hexagons correspond to the first Brillouin zone of bottom and top layers, respectively, and thick small-hexagon to the MBZ. In MBZ, open and filled circles are two inequivalent $K$ points, red dots are equivalent points of $\bar{\Gamma}$ point, and blue dots are equivalent points of $M$ point.

### A. $\bar{\Gamma}$ Point

There are in total three pairs of opposite momenta, denoted as $\pm\boldsymbol{\Lambda}_{a=1,2,3}$, which are located closest to the original Dirac points $\pm\boldsymbol{K}_{1,2}$ of individual graphene layers *and* fold onto $\bar{\Gamma}$ of MBZ. These three $\Lambda$ points are all integer multiples of the two superlattice reciprocal vectors $\boldsymbol{G}_{1,2} = G_\theta\left(\pm\frac{1}{2}, -\frac{\sqrt{3}}{2}\right), G_\theta = \frac{8\pi}{\sqrt{3}a}\sin\frac{\theta}{2}$, and related by three-fold rotation symmetry, as shown in Fig. 2. Compare with the maintext $\boldsymbol{G}_1 = \boldsymbol{G}_1^{\rm M} + \boldsymbol{G}_2^{\rm M}, \quad \boldsymbol{G}_2 = \boldsymbol{G}_1^{\rm M}$.

Interlayer tunneling leads to scatterings among $\pm\Lambda$ points on layer 1 and those on layer 2. Among all possible scattering processes, intervalley scattering between $+\Lambda$ points to $-\Lambda$ points requires large momentum transfer, hence is negligibly small when the twist angle is small. Thus we only consider intravalley scattering within the three $+\Lambda$ points that are all close to the original Dirac points $+\boldsymbol{K}_{1,2}$, and drop the valley index. Since we focus on $+\boldsymbol{K}_{1,2}$ valleys, we only need to consider two out of the four lowest energy eigenstates at $\bar{\Gamma}$ point, which are denoted by $\Psi_e^{\bar{\Gamma}}$ on electron side and $\Psi_e^{\bar{\Gamma}}$ on hole side. The other two lowest energy eigenstates coming from $-\boldsymbol{K}_{1,2}$ valleys will be time-reversal partners of $\Psi_{e,h}^{\bar{\Gamma}}$.

According to our discussion above, to the lowest order approximation, energy eigenstates at $\bar{\Gamma}$ are in general superpositons of $\xi_{\boldsymbol{k}}^m, \eta_{\boldsymbol{k}}^n$ where $\boldsymbol{k} = \boldsymbol{\Lambda}_a \quad (a = 1, 2, 3)$. While the energy spectrum depends on the form of tunneling operator $T(\boldsymbol{x}^m, \boldsymbol{y}^n)$, we now deduce purely from general symmetry considerations the essential form of these wavefunctions.

Any energy eigenstate at $\bar{\Gamma}$ must belong to one of the six irreducible representations of the point group $D_6$: four one-dimensional representations $A_1, A_2, B_1, B_2$, and two two-dimensional representation $E_1, E_2$. The two-fold rotation $C_{2y}$ around $y$-axis maps $+\boldsymbol{K}_{1,2}$ to $-\boldsymbol{K}_{2,1}$ respectively, i.e., simultaneously interchanges the two valleys and the two layers. Therefore, its action cannot be represented within the subspace of states around one valley. Thus it suffices to consider the subgroup $D_3$ that is generated by $C_{3z}$ and $C_{2x}$, and acts within $+\Lambda$ states belonging to the $+\boldsymbol{K}$ valley.

The subgroup $D_3$ hosts three irreducible representations $A_1, A_2$ and $E$, among which $A_1, A_2$ are 1D representations and can be labeled by the eigenvalue of angular momentum $L_z = 0$ while $E$ is 2D representation whose basis states can be labeled by $L_z = \pm 1$. According to group theory, an eigenstate $\Psi$ with angular momentum $L_z$ formed by Bloch states from three $\Lambda$ points can be generally written as

$$\Psi^{\bar{\Gamma}} = \sum_m \sum_{\boldsymbol{x}^m} \alpha_m \sum_{a=1}^{3} e^{i\boldsymbol{\Lambda}_a \cdot \boldsymbol{x}^m + \frac{2i}{3} a L_z \pi} \xi(\boldsymbol{x}^m) + \sum_n \sum_{\boldsymbol{y}^n} \beta_n \sum_{a=1}^{3} e^{i\boldsymbol{\Lambda}_a \cdot \boldsymbol{y}^n + \frac{2i}{3} a L_z \pi} \eta(\boldsymbol{y}^n) \tag{2}$$

where $\alpha_m, \beta_n$ are complex coefficients. Without loss of generality in the following we shall consider the energy eigenstate of the conduction mini-band, denoted by $\Psi_e^{\bar{\Gamma}}$. The analysis of the valence mini-band $\Psi_h^{\bar{\Gamma}}$ is similar.

We first focus on the case of $L_z = 0$. According to the general expression above, $\Psi^{\bar{\Gamma}}$ can be rewritten in the following suggestive way

$$\Psi^{\bar{\Gamma}} = e^{-i2\pi/3} \left[\alpha_A U^A(\boldsymbol{R}_c) + \alpha_B U^B(-\boldsymbol{R}_c)\right] + e^{i2\pi/3} \left[\beta_A L^A(-\boldsymbol{R}_c) + \beta_B L^B(\boldsymbol{R}_c)\right]. \tag{3}$$

Here $\boldsymbol{R}_c = \mathrm{L_M} \hat{\boldsymbol{x}}/\sqrt{3}$ is the coordinate of an BA spot closest to the AA spot at the origin. $U$ and $L$ are electron wavefunctions on the upper and lower layers respectively, defined by

$$U^m(\boldsymbol{R}) = \sum_{\boldsymbol{x}^m} e^{i\boldsymbol{K}_1 \cdot \boldsymbol{x}^m} f(\boldsymbol{x}^m - \boldsymbol{R}) \xi(\boldsymbol{x}^m), \tag{4}$$

$$L^n(\boldsymbol{R}) = \sum_{\boldsymbol{y}^n} e^{i\boldsymbol{K}_2 \cdot \boldsymbol{y}^n} f^*(\boldsymbol{y}^n - \boldsymbol{R}) \eta(\boldsymbol{y}^n). \tag{5}$$

Both $U, L$ are the product of intra-unit-cell wavefunction $e^{i\boldsymbol{K}\cdot\boldsymbol{r}}$ which is fast oscillating and the envelope function $f(\boldsymbol{r} - \boldsymbol{R})$ given by

$$f(\boldsymbol{r}) = e^{i(\boldsymbol{K}_1 - \boldsymbol{K}_2)\cdot\boldsymbol{r}} \times \left\{1 + e^{i\boldsymbol{G}_1\cdot\boldsymbol{r}} + e^{i\boldsymbol{G}_2\cdot\boldsymbol{r}}\right\}, \tag{6}$$

which is slowly varying. $f(\boldsymbol{r})$ is invariant under three-fold rotation around the origin.

Notice that this wavefunction has exactly the *same* envelope functions as that in $D_3$ structure formed by states near the same valley. Thus within continuum model which only considers envelope functions and neglects intervalley couplings, $D_3$ and $D_6$ structures share the same eigenstates at $\bar{\Gamma}$ point.

It is straightforward to show that the maxima of the envelop function $|f(\boldsymbol{r})|$ are located at AA spots $n_1\boldsymbol{A}_1 + n_2\boldsymbol{A}_2 \quad (n_{1,2} \in \mathbb{Z})$, which form a triangular lattice with primitive vectors $\boldsymbol{A}_{1,2} \equiv \mathrm{L_M}(\frac{\sqrt{3}}{2}, \pm\frac{1}{2})$. Compare with the maintext $\boldsymbol{A}_1 = \boldsymbol{L}_2^{\mathrm{M}} - \boldsymbol{L}_1^{\mathrm{M}}, \quad \boldsymbol{A}_2 = \boldsymbol{L}_1^{\mathrm{M}}$. Then, the maxima of $|f(\boldsymbol{r} \pm \boldsymbol{R}_c)|$ are located at the BA/AB spots $\mp\boldsymbol{R}_c + n_1\boldsymbol{A}_1 + n_2\boldsymbol{A}_2$, which also form a triangular lattice but shifted off the origin by $\mp\boldsymbol{R}_c$. Therefore, it follows from Eq. (3) that the component of Bloch wavefunction $\Psi^{\bar{\Gamma}}$ on the $A$ sublattice has its maxima at AB spots on layer 1 and at BA spots on layer 2, while the component on the $B$ sublattice has its maxima on BA spots on layer 1 and AB spots on layer 2.

This feature is robust and can be understood by symmetry considerations. We notice that both $A$ and $B$ sublattice sites do not coincide with rotation centers $n_1\boldsymbol{A}_1 + n_2\boldsymbol{A}_2$, where hexagon centers on two layers are registered, hence the intra-unit-cell phase factors already carry finite angular momenta. For $A$ sites, $e^{i\boldsymbol{K}_1\cdot\boldsymbol{x}^A}$ and $e^{i\boldsymbol{K}_2\cdot\boldsymbol{y}^A}$ have angular

momentum $-1$, and for $B$ sites, $e^{i\boldsymbol{K}_1\cdot\boldsymbol{x}^B}$ and $e^{i\boldsymbol{K}_2\cdot\boldsymbol{y}^B}$ have angular momentum $+1$. To make the total angular momentum $L_z=0$, the envelope functions of $A$ and $B$ sublattice wavefunctions must carry $\pm1$ angular momenta respectively.

For an envelope function carrying finite angular momentum, its amplitude should vanish at rotation centers $n_1\boldsymbol{A}_1+n_2\boldsymbol{A}_2$. Therefore, the maxima of both $A,B$-sublattice components of $\Psi^{\bar{\Gamma}}$ must be away from these AA spots. Furthermore, if there is only a single maximum within a supercell (as is the case here), this maximum can only be located at either AB or BA spots, because these positions are invariant under three-fold rotation with respect to AA spots up to superlattice translations. Finally, we note that under the combination of two-fold rotation $C_{2y}$ and time-reversal symmetry $T$, the two layers are interchanged, while the sublattice and angular momentum $L_z$ quantum numbers are unchanged. This implies that the maxima of $A$ sublattice wavefunction is symmetric under $C_{2y}$, hence must be located at AB spots on layer 1 and BA spots on layer 2, forming the $C_{2y}$ image of each other. Similarly, the maxima of $B$ sublattice wavefunction are located at BA spots on layer 1 and AB spots on layer 2.

Now we have $L_z=0$, hence the eigenstates are singlet and furnish 1D representations of $D_3$. Under $C_{2x}$, the wavefunction (2) splits into bonding ($A_1$) and antibonding ($A_2$) states. Taking into account $C_{2y}$ and another valley, we find four singlet eigenstates at $\bar{\Gamma}$ point, furnishing four different time-reversal-invariant 1D representations of $D_6$ as $c_{\mathrm{R}}\Psi^{\bar{\Gamma}}_{\mathrm{R}}+c^*_{\mathrm{R}}\bar{\Psi}^{\bar{\Gamma}}_{\mathrm{R}}$, where R$=A_1,B_1,A_2,B_2$ labels the representation, $c_{\mathrm{R}}\in\mathbb{C}$ is to be determined by microscopic details, $\bar{\Psi}$ denotes the time-reversal partner of $\Psi$, and the bare basis states are

$$\Psi^{\bar{\Gamma}}_{A1}=U^A(\boldsymbol{R}_c)+\bar{L}^A(-\boldsymbol{R}_c)+\bar{U}^B(-\boldsymbol{R}_c)+L^B(\boldsymbol{R}_c), \tag{7}$$
$$\Psi^{\bar{\Gamma}}_{B1}=U^A(\boldsymbol{R}_c)-\bar{L}^A(-\boldsymbol{R}_c)-\bar{U}^B(-\boldsymbol{R}_c)+L^B(\boldsymbol{R}_c), \tag{8}$$
$$\Psi^{\bar{\Gamma}}_{A2}=U^A(\boldsymbol{R}_c)-\bar{L}^A(-\boldsymbol{R}_c)+\bar{U}^B(-\boldsymbol{R}_c)-L^B(\boldsymbol{R}_c), \tag{9}$$
$$\Psi^{\bar{\Gamma}}_{B2}=U^A(\boldsymbol{R}_c)+\bar{L}^A(-\boldsymbol{R}_c)-\bar{U}^B(-\boldsymbol{R}_c)-L^B(\boldsymbol{R}_c). \tag{10}$$

We thus conclude that, to respect the symmetry group $D_6\times$U(1) of twisted bilayer graphene within continuum model, the energy eigenstate at $\bar{\Gamma}$ point with angular momentum $L_z=0$ has the same envelope functions as those in $D_3$ structure. This observation motivates us to consider honeycomb lattice formed by AB and BA spots in constructing effective tight-binding model for both $D_3$ and $D_6$ structure.

### B. $\bar{M}$ Point

For each $\bar{M}$ point, there are in total two momenta $\pm\frac{1}{2}(\boldsymbol{K}_1+\boldsymbol{K}_2)$, which are located closest to the original Dirac points $\pm\boldsymbol{K}_{1,2}$ of individual graphene layers *and* fold onto $\bar{M}$ of MBZ, whose little group is $D_2$. Denote $\boldsymbol{M}=\frac{1}{2}(\boldsymbol{K}_1+\boldsymbol{K}_2)$, then we can construct all four time-reversal-invariant 1D irreducible representations of $D_2$ by states at $\pm\boldsymbol{M}$ in both layers as follows

$$\Psi^{\bar{M}}_{A}=\alpha_0(\xi^A_M+\eta^B_M)+\alpha_0^*(\xi^B_M+\eta^A_M)+\alpha_0(\eta^A_{-M}+\xi^B_{-M})+\alpha_0^*(\eta^B_{-M}+\xi^A_{-M}), \tag{11}$$
$$\Psi^{\bar{M}}_{B1}=\alpha_1(\xi^A_M+\eta^B_M)-\alpha_1^*(\xi^B_M+\eta^A_M)-\alpha_1(\eta^A_{-M}+\xi^B_{-M})+\alpha_1^*(\eta^B_{-M}+\xi^A_{-M}), \tag{12}$$
$$\Psi^{\bar{M}}_{B2}=\alpha_2(\xi^A_M-\eta^B_M)+\alpha_2^*(\xi^B_M-\eta^A_M)+\alpha_2(\eta^A_{-M}-\xi^B_{-M})+\alpha_2^*(\eta^B_{-M}-\xi^A_{-M}), \tag{13}$$
$$\Psi^{\bar{M}}_{B3}=\alpha_3(\xi^A_M-\eta^B_M)-\alpha_3^*(\xi^B_M-\eta^A_M)-\alpha_3(\eta^A_{-M}-\xi^B_{-M})+\alpha_3^*(\eta^B_{-M}-\xi^A_{-M}), \tag{14}$$

with four complex coefficients $\alpha_i(i=0,1,2,3)$ to be determined by microscopic details.

### C. $\bar{K}$ Point

For $\bar{K}$ point, there are in total two momenta $\boldsymbol{K}_1,-\boldsymbol{K}_2$, which fold onto $\bar{K}$ of MBZ, whose little group is $D_3$. We can construct two 2D irreducible representations of $D_3$ by states at $\boldsymbol{K}_1,-\boldsymbol{K}_2$ in both layers as follows

$$\Psi^{\bar{K}}_1=(\xi^A_{K_1},\eta^A_{-K_2}),\quad \Psi^{\bar{K}}_2=(\eta^B_{-K_2},\xi^B_{K_1}). \tag{15}$$

## II. $D_3$ STRUCTURE

When the rotation center of TBG is the registered carbon atoms of two layers, the TBG has point group $D_3$ with respect to the rotation center. In this case the triangular lattice formed by AA spots and the honeycomb lattice

formed by AB and BA spots are both candidates for effective tight-binding model. Similar to above structures, in Table. IV we list band symmetries in triangular lattice model with different Wannier orbital symmetries, and in Table. V find out the correct effective-tight binding model to reproduce the realistic band symmetries. This case is the focus of the maintext.

| Lattice | Orbital | $\Gamma(D_3)$ | $K(D_3)$ | $M(C_2)$ | On-site | U(1) |
|---|---|---|---|---|---|---|
| Honeycomb | $s, p_z$ | $\{A_1; A_2\}$ | $E$ | $\{A; B\}$ | $A$ | $s \pm ip_z$ |
| $C_3$ | $(p_x, p_y)$ | $\{E; E\}$ | $\{A_1, A_2, E\}$ | $\{A, B; A, B\}$ | $E$ | $p_x \pm ip_y$ |
| Triangular | $s$ | $A_1$ | $A_1$ | $A$ | $A_1$ | $s \pm ip_z$ |
| $D_3$ | $p_z$ | $A_2$ | $A_2$ | $B$ | $A_2$ | $s \pm ip_z$ |
| | $(p_x, p_y)$ | $E$ | $E$ | $\{A, B\}$ | $E$ | $p_x \pm ip_y$ |

TABLE IV: Symmetries of eigenstates at $\Gamma, K, M$ points in different tight-binding models.

| | $\bar{\Gamma}$ | $\bar{K}$ | $\bar{M}$ | Orbitals | Lattice and U(1) |
|---|---|---|---|---|---|
| Group | $D_3$ | $D_3$ | $C_2$ | $C_3$ | Honeycomb |
| Reps | $\{E; E\}$ | $\{A_1, A_2, E\}$ | $\{A, B; A, B\}$ | $(p_x, p_y)$ | $p_x \pm ip_y$ |

TABLE V: Symmetries of lowest four eigenstates at $\bar{\Gamma}, \bar{K}, \bar{M}$ points for $D_3$ structure of TBG.

As shown in previous section, in $D_3$ and $D_6$ superlattice structures with the same twist angle, eigenstates at a given high-symmetry point are formed by basis states with exactly the *same* envelope functions. Thus within continuum model which only considers envelope functions and neglects intervalley couplings, at any given high-symmetry point, $D_3$ and $D_6$ structures share the same envelope functions of basis states, while eigenstates can be different combinations of basis states according to different point group symmetry. We can find such different combinations from realistic band structures. As a concrete example, we compare $\Gamma$ point eigenstates in $D_3$ and $D_6$ structures at commensurate angle $\theta = 1.08°$ through microscopic tight-binding calculations.

In Fig. 3, we compare valley-conserving states $\Psi_\xi^{\overline{\Gamma}}(x,y)$ at $\overline{\Gamma}$ point with the same eigenenergy but in different lattice structures. These valley-conserving states are superpositions of $\overline{\Gamma}$ point eigenstates, which are also eigenstates in $D_3$ case while not in $D_6$ case. Here we focus on the states from valley $\xi = +1$. The main difference lies in the in-plane rotation symmetry of $\Psi_\xi^{\overline{\Gamma}}(x,y)$, which can be found from the phase distribution. In $D_6$ structure, $\Psi_\xi^{\overline{\Gamma}}(x,y)$ has sixfold rotation symmetry with angular momentum $L_z = 3 \pmod 6$, while in $D_3$ structure $\Psi_\xi^{\overline{\Gamma}}(x,y)$ has only threefold rotation symmetry with angular momentum $L_z = -\xi = -1 \pmod 3$. To calculate $\Psi_\xi^{\overline{\Gamma}}(x,y)$ we employ the microscopic tight-binding model of commensurate twisted bilayer graphenes. The hopping between two carbon atoms separated by vector $\mathbf{R}$ is described by the Slater-Koster integral

$$-t(\mathbf{R}) = V_{pp\pi}\left[1-\left(\frac{\mathbf{R}\cdot\mathbf{e}_z}{R}\right)^2\right] + V_{pp\sigma}\left(\frac{\mathbf{R}\cdot\mathbf{e}_z}{R}\right)^2, \quad V_{pp\pi} = V_{pp\pi}^0 e^{-(R-a_0)/r_0}, \; V_{pp\sigma} = V_{pp\sigma}^0 e^{-(R-d_0)/r_0}. \tag{16}$$

Here $\mathbf{e}_z$ is the unit vector perpendicular to the graphene plane, $a_0 = a/\sqrt{3} \approx 0.142\,\text{nm}$ is the distance of neighboring $A$ and $B$ sites on graphene, and $d_0 \approx 0.335\,\text{nm}$ is the uniform interlayer spacing of the flat twisted bilayer graphene. The parameter $V_{pp\pi}^0$ is the transfer integral between the nearest-neighbor atoms on graphene, and $V_{pp\sigma}^0$ is the transfer integral between vertically located atoms on the neighboring layers of graphite. We take $V_{pp\pi}^0 \approx -2.7\,\text{eV}$, $V_{pp\sigma}^0 \approx 0.48\,\text{eV}$, to fit the dispersions of monolayer graphene. Here $r_0$ is the decay length of the transfer integral, and is chosen as $0.184a$ so that the next nearest intralayer coupling becomes $0.1V_{pp\pi}^0$.

The commensurate twist angle $\theta$ satisfies

$$\cos\theta = \frac{3n^2+3n+1/2}{3n^2+3n+1}, \quad n \in \mathbb{N} \tag{17}$$

and we choose $n = 30$ such that $\theta = 1.08°$. The moiré lattice constant is 12.99 nm and each supercell contains $4(3n^2+3n+1)$ =11164 carbon atoms.

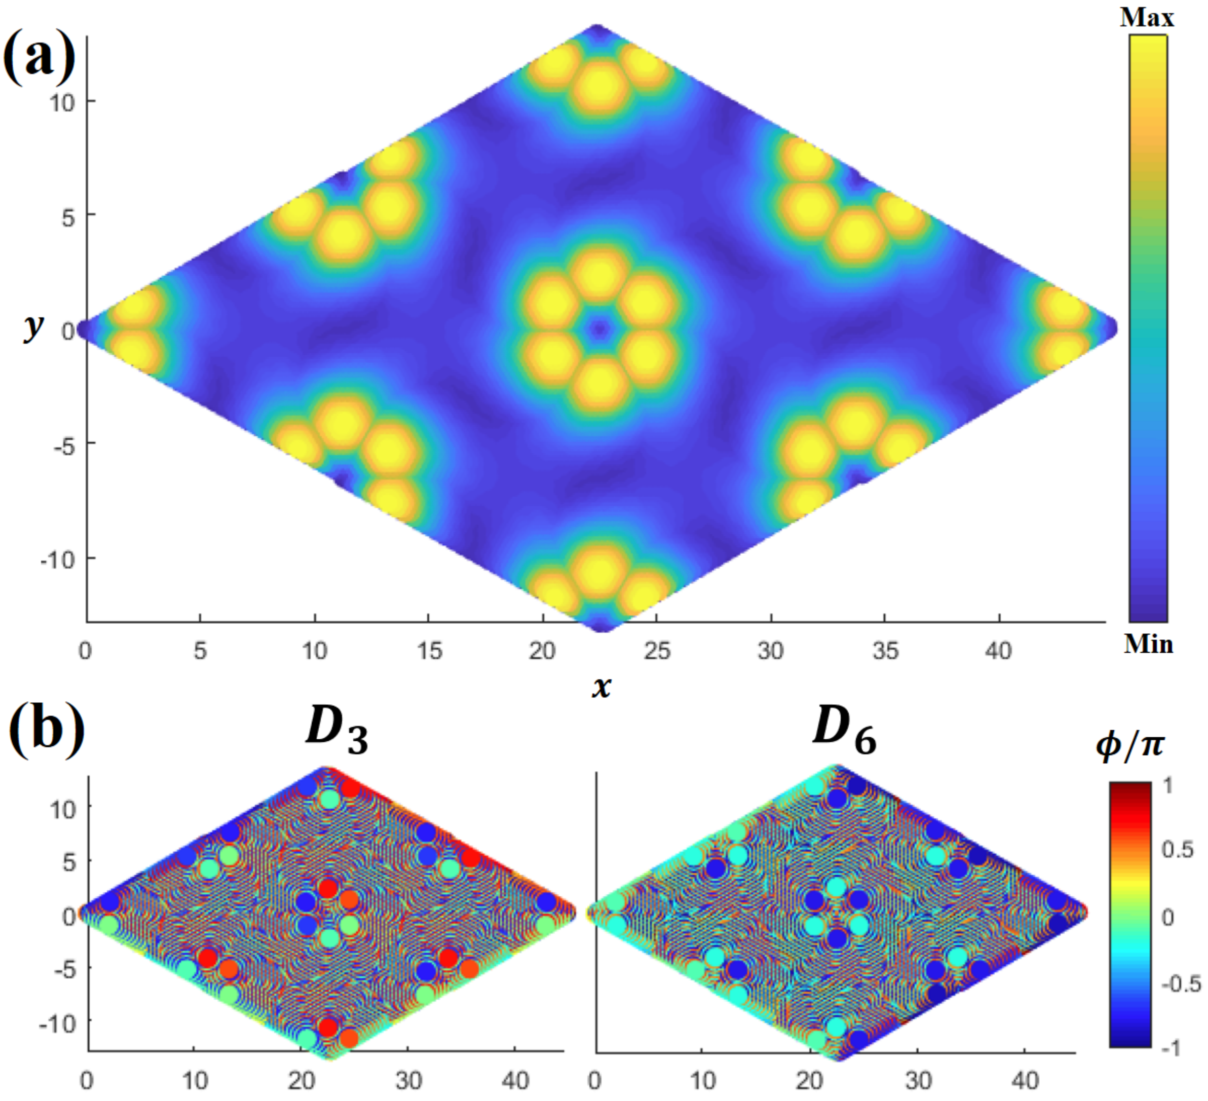


FIG. 3: The spatial distributions of (a) amplitude and (b) phase of valley-conserving state $\Psi_\xi^{\overline{\Gamma}}(x, y)$ at $\overline{\Gamma}$ point in twist bilayer graphene (TBG) at commensurate twist angle 1.08° but with different point groups $D_3$ and $D_6$ respectively. Here $\xi = +1$ and only the component in layer 1 is plotted for clearness. At this angle, the band width at $\overline{\Gamma}$ point is $W$ =20 meV, with hole side at energy $E = 0.1372$ eV. In $D_3$ case, we construct $\Psi_\xi^{\overline{\Gamma}}(x, y)$ from a linear combination out of the doublet eigenstates on the hole side with energy $E$. In $D_6$ case we construct $\Psi_\xi^{\overline{\Gamma}}(x, y)$ from a linear combination of two singlet eigenstates on the hole side at energy $E \pm \delta/2$ respectively, where $\delta = 0.8\mu$eV denotes intervalley coupling. The probability distributions $|\Psi_{\xi,1}^{\overline{\Gamma}}(x, y)|^2$ at layer 1 are the same for $D_3$ and $D_6$ cases and plotted in a). The phase distributions $\phi(x, y) \equiv \text{Arg}\left[\Psi_{\xi,1}^{\overline{\Gamma}}(x, y)\right]$ at layer 1 are plotted in (a) for $D_3$ and $D_6$ cases respectively. From phase distributions in (b) we can identify the rotation symmetry and hence angular momentum of $\Psi_\xi^{\overline{\Gamma}}(x, y)$ for the two cases. The unit of $x, y$-axes is nm, and the moiré lattice constant is 12.99 nm.

## III. $D_2$ STRUCTURE

When the rotation center of TBG is the registered carbon-bond midpoints of two layers, the TBG has point group $D_2$ with respect to the rotation center. Similar to $C_2$ structure, threefold rotation is lost and the triangular lattice formed by AA spots is the only choice for effective tight-binding model. In Table. VI we list band symmetries in triangular lattice model with different Wannier orbital symmetries, and in Table. VII find out the correct effective-tight binding model to reproduce the realistic band symmetries.

Furthermore, the orbital U(1) symmetry is also respected. From continuum model we know $C_{2y}$ should flip the

| Orbital | $\bar{\Gamma}(D_2)$ | $\bar{K}(C_2)$ | $\bar{M}(D_2)$ |
|---|---|---|---|
| $s$ | $A$ | $A$ | $A$ |
| $p_x$ | $B_1$ | $B$ | $B_1$ |
| $p_y$ | $B_2$ | $A$ | $B_2$ |
| $p_z$ | $B_3$ | $B$ | $B_3$ |

TABLE VI: Symmetries of eigenstates at $\bar{\Gamma}, \bar{K}, \bar{M}$ points in tight-binding models with different orbitals (Orbital) on the triangular lattice formed by AA spots. The underlying TBG is $D_2$ structure.

| | $\bar{\Gamma}$ | $\bar{K}$ | $\bar{M}$ | Orbitals | Lattice and U(1) |
|---|---|---|---|---|---|
| Group | $D_2$ | $C_2$ | $D_2$ | $D_2$ | Triangular |
| Reps | $\{A, B_1; B_2, B_3\}$ | $\{A, B; A, B\}$ | $\{A, B_1; B_2, B_3\}$ | $\{s, p_x; p_y, p_z\}$ | $s \pm ip_x; p_y \pm ip_z$ |

TABLE VII: Symmetries of lowest four eigenstates at $\bar{\Gamma}, \bar{K}, \bar{M}$ points for $D_2$ structure of TBG.

valley index, and hence the basis constructed for orbital U(1) symmetry should become complex conjugate under $C_{2y}$.

### A. Eigenstates at High-Symmetry Points

To see the microscopic composition of eigenstates at high symmetry points in $D_2$ structure, we carry out similar study of the lowest minibands of TBG at $\bar{\Gamma}, \bar{M}, \bar{K}$ points of the MBZ, as in previous section.

The eigenstates at $\bar{\Gamma}$ of MBZ furnish four different time-reversal-invariant 1D representations of $D_2$ as $a_{\rm R}\Psi^{\bar{\Gamma}}_{\rm R}+a^*_{\rm R}\bar{\Psi}^{\bar{\Gamma}}_{\rm R}$, where R$=A, B_1, B_2, B_3$ labels the representation, $a_{\rm R} \in \mathbb{C}$ is to be determined by microscopic details, $\bar{\Psi}$ denotes the time-reversal partner of $\Psi$, and the bare basis states are

$$\Psi^{\bar{\Gamma}}_{A} = U^A(\boldsymbol{R}_c) + \bar{L}^A(-\boldsymbol{R}_c) + \bar{U}^B(-\boldsymbol{R}_c) + L^B(\boldsymbol{R}_c), \tag{18}$$
$$\Psi^{\bar{\Gamma}}_{B1} = U^A(\boldsymbol{R}_c) - \bar{L}^A(-\boldsymbol{R}_c) - \bar{U}^B(-\boldsymbol{R}_c) + L^B(\boldsymbol{R}_c), \tag{19}$$
$$\Psi^{\bar{\Gamma}}_{B2} = U^A(\boldsymbol{R}_c) + \bar{L}^A(-\boldsymbol{R}_c) - \bar{U}^B(-\boldsymbol{R}_c) - L^B(\boldsymbol{R}_c), \tag{20}$$
$$\Psi^{\bar{\Gamma}}_{B3} = U^A(\boldsymbol{R}_c) - \bar{L}^A(-\boldsymbol{R}_c) + \bar{U}^B(-\boldsymbol{R}_c) - L^B(\boldsymbol{R}_c). \tag{21}$$

The little group of $\bar{M}$ is $D_2$ as in $D_6$ case. Similarly, we can construct all four time-reversal-invariant 1D irreducible representations of $D_2$ by states at $\pm\boldsymbol{M}$ in both layers as follows

$$\Psi^{\bar{M}}_{A} = \alpha_0(\xi^A_M + \eta^B_M) + \alpha^*_0(\xi^B_M + \eta^A_M) + \alpha_0(\eta^A_{-M} + \xi^B_{-M}) + \alpha^*_0(\eta^B_{-M} + \xi^A_{-M}), \tag{22}$$
$$\Psi^{\bar{M}}_{B1} = \alpha_1(\xi^A_M + \eta^B_M) - \alpha^*_1(\xi^B_M + \eta^A_M) - \alpha_1(\eta^A_{-M} + \xi^B_{-M}) + \alpha^*_1(\eta^B_{-M} + \xi^A_{-M}), \tag{23}$$
$$\Psi^{\bar{M}}_{B2} = \alpha_2(\xi^A_M - \eta^B_M) + \alpha^*_2(\xi^B_M - \eta^A_M) + \alpha_2(\eta^A_{-M} - \xi^B_{-M}) + \alpha^*_2(\eta^B_{-M} - \xi^A_{-M}), \tag{24}$$
$$\Psi^{\bar{M}}_{B3} = \alpha_3(\xi^A_M - \eta^B_M) - \alpha^*_3(\xi^B_M - \eta^A_M) - \alpha_3(\eta^A_{-M} - \xi^B_{-M}) + \alpha^*_3(\eta^B_{-M} - \xi^A_{-M}), \tag{25}$$

with four complex coefficients $\alpha_i (i = 0, 1, 2, 3)$ to be determined by microscopic details.

For $\bar{K}$ point, the little group is now $C_2$. We can construct 1D irreducible representations of $C_2$ by states at $\boldsymbol{K}_1, -\boldsymbol{K}_2$ in both layers as follows

$$\Psi^{\bar{K}}_{A} = \xi^A_{\boldsymbol{K}_1} + \eta^A_{-\boldsymbol{K}_2}, \quad \tilde{\Psi}^{\bar{K}}_{A} = \xi^B_{\boldsymbol{K}_1} + \eta^B_{-\boldsymbol{K}_2}, \quad \Psi^{\bar{K}}_{B} = \xi^A_{\boldsymbol{K}_1} - \eta^A_{-\boldsymbol{K}_2}, \quad \tilde{\Psi}^{\bar{K}}_{B} = \xi^B_{\boldsymbol{K}_1} - \eta^B_{-\boldsymbol{K}_2}. \tag{26}$$

## IV. $C_2$ STRUCTURE

When the rotation center of TBG is not among the three types of high-symmetry points discussed above, the TBG has point group $C_2$ with respect to the rotation center. In this case threefold rotation is lost and the triangular lattice formed by AA spots is the only choice for effective tight-binding model. In Table. VIII we list band symmetries with different Wannier orbital symmetries, and in Table. IX we list band symmetries obtained from realistic tight-binding calculations and find out the correct effective-tight binding model to reproduce them.

The orbital U(1) symmetry is found respected. From continuum model we know $C_{2y}$ should flip the valley index, and hence the basis constructed for orbital U(1) symmetry should become complex conjugate under $C_{2y}$.

| Orbital | $\bar{\Gamma}(C_2)$ | $\bar{K}(C_2)$ | $\bar{M}(C_2)$ |
|---|---|---|---|
| $s, p_y$ | $A$ | $A$ | $A$ |
| $p_x, p_z$ | $B$ | $B$ | $B$ |

TABLE VIII: Symmetries of eigenstates at $\bar{\Gamma}, \bar{K}, \bar{M}$ points in tight-binding models with different orbitals (Orbital) on the triangular lattice formed by AA spots. The underlying TBG is $C_2$ structure.

| | $\bar{\Gamma}$ | $\bar{K}$ | $\bar{M}$ | Orbitals | Lattice and U(1) |
|---|---|---|---|---|---|
| Group | $C_2$ | $C_2$ | $C_2$ | $C_2$ | Triangular |
| Reps | $\{A, B; A, B\}$ | $\{A, B; A, B\}$ | $\{A, B; A, B\}$ | $\{s, p; s, p\}$ | $s \pm ip$ |

TABLE IX: Symmetries of lowest four eigenstates at $\bar{\Gamma}, \bar{K}, \bar{M}$ points for $C_2$ structure of TBG. Wannier orbitals (Orbitals) and lattices (Lattice) in effective tight-binding models are also shown. At each high symmetry point, the little group (Group) and irreducible representations (Reps) of the lowest four bands are listed, the semicolons are used to separate conduction and valence bands when they are separable. For Wannier orbitals, Group is the point group with respect to AA spots, Reps are real representations furnished by Wannier orbitals. In the last column, Wannier orbitals preserving orbital U(1) symmetry are also shown. Here $p$ orbital in $C_2$ structure can be $p_x$ or $p_z$, which is odd under $C_{2y}$.

### A. Eigenstates at High-Symmetry Points

To see the microscopic composition of eigenstates at high symmetry points in $C_2$ structure, we carry out similar study of the lowest minibands of TBG at $\bar{\Gamma}, \bar{M}, \bar{K}$ points of the MBZ, as in previous sections. Since $C_2$ structure has the lowest symmetry, the eigenstates obtained in $D_2$ structure will simply apply with the same form, while some states now belong to the same representation due to symmetry reduction. In this case The little group of $\bar{\Gamma}, \bar{K}, \bar{M}$ is the same $C_2$.

The eigenstates at $\bar{\Gamma}$ of MBZ furnish four different time-reversal-invariant 1D representations of $C_2$ as $\lambda_{\rm R}\Psi_{\rm R}^{\bar{\Gamma}}+\lambda_{\rm R}^*\bar{\Psi}_{\rm R}^{\bar{\Gamma}}$, where R=$A, B$ labels the representation, $\lambda_{\rm R} \in \mathbb{C}$ is to be determined by microscopic details, $\bar{\Psi}$ denotes the time-reversal partner of $\Psi$, and the bare basis states are

$$\Psi_A^{\bar{\Gamma}} = U^A(\boldsymbol{R}_c) + \bar{L}^A(-\boldsymbol{R}_c) + \bar{U}^B(-\boldsymbol{R}_c) + L^B(\boldsymbol{R}_c), \tag{27}$$
$$\Psi_B^{\bar{\Gamma}} = U^A(\boldsymbol{R}_c) - \bar{L}^A(-\boldsymbol{R}_c) - \bar{U}^B(-\boldsymbol{R}_c) + L^B(\boldsymbol{R}_c), \tag{28}$$
$$\tilde{\Psi}_A^{\bar{\Gamma}} = U^A(\boldsymbol{R}_c) + \bar{L}^A(-\boldsymbol{R}_c) - \bar{U}^B(-\boldsymbol{R}_c) - L^B(\boldsymbol{R}_c), \tag{29}$$
$$\tilde{\Psi}_B^{\bar{\Gamma}} = U^A(\boldsymbol{R}_c) - \bar{L}^A(-\boldsymbol{R}_c) + \bar{U}^B(-\boldsymbol{R}_c) - L^B(\boldsymbol{R}_c). \tag{30}$$

Similarly, we can construct all four time-reversal-invariant 1D irreducible representations at $\pm\boldsymbol{M}$ in both layers as follows

$$\Psi_A^{\bar{M}} = \alpha_0(\xi_M^A + \eta_M^B) + \alpha_0^*(\xi_M^B + \eta_M^A) + \alpha_0(\eta_{-M}^A + \xi_{-M}^B) + \alpha_0^*(\eta_{-M}^B + \xi_{-M}^A), \tag{31}$$
$$\Psi_B^{\bar{M}} = \alpha_1(\xi_M^A + \eta_M^B) - \alpha_1^*(\xi_M^B + \eta_M^A) - \alpha_1(\eta_{-M}^A + \xi_{-M}^B) + \alpha_1^*(\eta_{-M}^B + \xi_{-M}^A), \tag{32}$$
$$\tilde{\Psi}_A^{\bar{M}} = \alpha_2(\xi_M^A - \eta_M^B) + \alpha_2^*(\xi_M^B - \eta_M^A) + \alpha_2(\eta_{-M}^A - \xi_{-M}^B) + \alpha_2^*(\eta_{-M}^B - \xi_{-M}^A), \tag{33}$$
$$\tilde{\Psi}_B^{\bar{M}} = \alpha_3(\xi_M^A - \eta_M^B) - \alpha_3^*(\xi_M^B - \eta_M^A) - \alpha_3(\eta_{-M}^A - \xi_{-M}^B) + \alpha_3^*(\eta_{-M}^B - \xi_{-M}^A), \tag{34}$$

with four complex coefficients $\alpha_i (i = 0, 1, 2, 3)$ to be determined by microscopic details.

For $\bar{K}$ point, we can construct 1D irreducible representations of $C_2$ by states at $\boldsymbol{K}_1, -\boldsymbol{K}_2$ in both layers as follows

$$\Psi_A^{\bar{K}} = \xi_{\boldsymbol{K}_1}^A + \eta_{-\boldsymbol{K}_2}^A, \quad \tilde{\Psi}_A^{\bar{K}} = \xi_{\boldsymbol{K}_1}^B + \eta_{-\boldsymbol{K}_2}^B, \quad \Psi_B^{\bar{K}} = \xi_{\boldsymbol{K}_1}^A - \eta_{-\boldsymbol{K}_2}^A, \quad \tilde{\Psi}_B^{\bar{K}} = \xi_{\boldsymbol{K}_1}^B - \eta_{-\boldsymbol{K}_2}^B. \tag{35}$$

As a result, we find that in all the different superlattice structures with the same twist angle, eigenstates at a given high-symmetry point are formed by basis states with exactly the *same* envelope functions. Thus within continuum model which only considers envelope functions and neglects intervalley couplings, at any given high-symmetry point, $C_2, D_2, D_3$ and $D_6$ structures share the same envelope functions of basis states, while eigenstates can be different combinations of basis states according to different point group symmetry.

### B. Effective Tight-Binding Model

Both conduction and valence bands can be described by $s, p$ orbitals in a triangular lattice formed by AA spots. Here the $p$ orbital is odd under $C_{2y}$ and can be $p_x$ or $p_z$. Together, the conduction and valence band structure can be described by exactly the same two-orbital model on the *honeycomb* lattice (formed by two triangular lattices) as in the maintext

$$H = \sum_{\xi=\pm}\sum_{ij} t(\boldsymbol{r}_{ij}) e^{i\xi\phi(\boldsymbol{r}_{ij})} c^\dagger_{i\xi} c_{j\xi} \tag{36}$$

where the only difference is that the valley-conserving orbital is $c_{j\xi} = (s_j + i\xi p_j)/\sqrt{2}$ at site $j$, and $s_j, p_j$ are associated with $s, p$ orbitals respectively. The symmetry group of this model is $\mathcal{G} = C_2\times\mathrm{U}(1)\times\mathrm{SU}(2)\times T$ where the point group of TBG ($C_2$) acts jointly on lattice sites and $s, p$ orbitals, and the rest symmetries are the same as before. To capture key features in the band structure, we keep dominate terms in Hamiltonian (36) and obtain the minimum model, as we did in the maintext

$$H_0 = -\mu\sum_i (s^\dagger_i s_i + p^\dagger_i p_i) + \sum_{\langle ij\rangle} t_1(s^\dagger_i s_j + p^\dagger_i p_j) + \sum_{\langle ij\rangle'} \tilde{t}_2(s^\dagger_i s_j + p^\dagger_i p_j) + t'_2(s^\dagger_i p_j - p^\dagger_i s_j) + h.c. \tag{37}$$

where $\tilde{t}_2, t'_2$ are real hopping parameters for fifth-nearest neighbors, and the sum over $\langle ij\rangle'$ includes bonds with length $\sqrt{3}L_{\mathrm{M}}$ along three directions $\hat{\boldsymbol{x}}, C_{3z}\hat{\boldsymbol{x}}$ and $C^2_{3z}\hat{\boldsymbol{x}}$. Since all hopping parameters are real in the basis of real orbitals, the minimum model is time-reversal invariant. The orbital U(1) symmetry becomes SO(2) symmetry in terms of real $s, p$ orbitals, and thus only inner product or cross product of $s, p$ orbitals are allowed in minimum model. The intra-orbital hopping terms have the form of inner product of $s, p$ orbitals and preserve SU(4) symmetry in orbital and spin space. The inter-orbital hopping term has the form of cross product of $s, p$ orbitals and break SU(4) down to U(1)$\times$SU(2). Under $C_{2y}$, the index $i, j$ in fifth-nearest-neighbor hopping $s^\dagger_i p_j - p^\dagger_i s_j$ are interchanged, $s, p$ map to $s, -p$ respectively, and as a result inter-orbital hopping between fifth-nearest neighbors is invariant. In other words, minimum model (37) preserves symmetry group $\mathcal{G}$, and similar arguments can be carried out to for the full effective model (36). Notice that in this case threefold rotation is lost and $A, B$ sublattices in the honeycomb lattice can form bonding and antibonding states such that the two-orbital honeycomb lattice model is essentially a four-orbital triangular lattice model.

At the same twist angle, within continuum model $C_2, D_2, D_3$ and $D_6$ structures share the same energy dispersion. The tiny energy differences ($\sim\mu$eV) in band structures between different superlattice structures are due to intervalley coupling, which is beyond continuum model. In $D_3$ lattice structure, the intervalley coupling can only be realized in effective tight-binding model by hopping between $p_+$ and $p_-$ orbitals,while in $C_2$ and $D_2$ structures intervalley coupling can allow different on-site energy terms for different singlet Wannier orbitals.
